# Supplementary material for: Development of a Two-Level ML Spatial-temporal Framework for Industrial Thermal Striping Applications
Source: arXiv:2301.05667 source file (2023-05-30)
Supplement: Supplementary file 1 [file appendix.tex]

\section*{Appendix: Hyperparameter Tuning}
